# Supplementary material for: Anomalous mirror symmetry breaking in a model insulating cuprate Sr$_2$CuO$_2$Cl$_2$
Source: arXiv:2008.06516 source file (2020-08-14)
Supplement: Supplementary file 1 [file BRR_SOM_8-5-2020.pdf]

# SUPPLEMENTARY INFORMATION

# Anomalous mirror symmetry breaking in a model insulating cuprate $Sr_2CuO_2Cl_2$

A. de la Torre,[1,2] K. L. Seyler,[1,2] L. Zhao,[3] S. Di Matteo,[4] M. S. Scheurer,[5] Y. Li,[6] B. Yu,[6] M. Greven,[6] S. Sachdev,[5] M. R. Norman,[7] and D. Hsieh,[1,2]

**CONTENTS**

1. **Mathematical expressions for SHG processes**
2. **Comparison to GaAs**
3. **Simulated RA-SHG patterns using AFM point group**
4. **Description of possible $A_{2g}$ order parameters**
5. **Temperature dependence of normal incidence intensity**
6. **Temperature dependence of intensity in PS and PP channels**
7. **Temperature and φ-dependence of intensity in SP and PP channels**
8. **Effects of non-uniform lattice contraction**
9. **Laser fluence and average power considerations**
10. **Effects of thermal cycling**
11. **Discussion of the effects of crystal imperfections**
12. **Comparison to prior SHG work on YBCO**

## 1. Mathematical expressions for SHG processes

Table S1 summarizes all of the SHG processes discussed in our work and our physical motivation for considering them. In addition, we also included MD and EQ SHG from the inversion preserving $4'/mmm'$ point group, which describes the $\Theta_I$ loop current phase proposed by Varma[1]. As shown in Table S2, this is not consistent with our data. Note that ED, MD and EQ refer to the following processes respectively: $P_i^{2\omega} = \chi_{ijk}^{ED} E_j^{\omega} E_k^{\omega}$ , $P_i^{2\omega} = \chi_{ijk}^{MD} E_j^{\omega} H_k^{\omega}$ and $P_i^{2\omega} = \chi_{ijkl}^{EQ} E_j^{\omega} \nabla_k E_l^{\omega}$ . The structure of the SHG susceptibility tensor associated with each process and point group is represented by a letter followed by a number (e.g. *H*3), in accordance with the nomenclature used by Birss (Ref. 2). Explicit forms of these tensors are listed later on, together with expressions for the RA-SHG pattern calculated in all four polarization channels PP, SP, PS and SS.

**Table S1: Summary of SHG processes considered in this work.**

| Point group | ED | MD | EQ | Physical origin |
|---|---|---|---|---|
| **4/*mmm*** | --- | *H3* | *H4* | Reported crystal structure |
| **4*mm*** | *I3* | *Not shown* | *Not shown* | Surface of 4/*mmm* |
| ***mmm*1′** | --- | *D3* | *D4* | Reported AFM structure |
| ***mm*21′** | *E3* | *Not shown* | *Not shown* | Surface of *mmm*1′ |
| **4/*m*** | --- | *F3* | *F4* | Candidate structure for $T < T_N$ |
| **4/*mm′m′*** | --- | *H3/I3*(*c*) | *H4/I4*(*c*) | $A_{2g}$ magnetic order |
| **4′/*mmm′*** | --- | *H3/J3*(*c*) | *H4/J4*(*c*) | Varma $\Theta_I$ loop current order [1] |

For magnetic point groups, unless indicated, *c*-type (time-reversal odd) and *i*-type (time-reversal even) tensors have the same expressions. The symbol --- means the process is forbidden. For inversion broken point groups, we only consider the dominant ED contribution.

Table S2 summarizes the dependence of the SHG intensity on the incident angle θ and scattering plane angle φ for all considered processes and point groups in each of the four polarization channels. Importantly, only the MD(c) process from a 4/*mm′m′* point group has a forbidden response in the PS and SS channels, which is necessary to explain our data. We also note that the clear θ-dependence we observe in the SS channel immediately rules out an ED process. Therefore no bulk inversion broken point groups are considered.

**Table S2: Summary of angular dependences of SHG processes**

| Point group | Process | PP | SP | PS | SS |
|---|---|---|---|---|---|
| **4/*mmm*** | MD | θ | θ | --- | --- |
| **4/*mmm*** | EQ | θ , φ | θ , φ | θ , φ | θ , φ |
| **4*mm*** | ED | θ | θ | --- | --- |
| ***mmm*1′** | MD (*i*/*c*) | θ , φ | θ , φ | θ , φ | θ , φ |
| ***mmm*1′** | EQ (*i*/*c*) | θ , φ | θ , φ | θ , φ | θ , φ |
| ***mm*21′** | ED (*i*/*c*) | θ , φ | θ , φ | θ , φ | --- |
| **4/*m*** | MD | θ | θ | θ | θ |
| **4/*m*** | EQ | θ , φ | θ , φ | θ , φ | θ , φ |
| **4/*mm′m′*** | MD (*c*) | --- | --- | θ | θ |
| **4/*mm′m′*** | EQ (*c*) | θ , φ | θ , φ | θ , φ | θ , φ |
| **4′/*mmm′*** | MD (*c*) | θ , φ | θ , φ | θ , φ | θ , φ |
| **4′/*mmm′*** | EQ (*c*) | θ , φ | θ , φ | θ , φ | θ , φ |

Symbol definitions: (θ , φ) means depends on both θ and φ, (θ) means depends only on θ, (---) means forbidden. Detailed dependences on θ and φ are provided below in this section.

## ED tensors

*E3*, $\{\boldsymbol{mm21'}\}$

$$\chi_{ijk}^{ED} = \begin{pmatrix} \begin{pmatrix} 0 \\ 0 \\ xxz \end{pmatrix} & \begin{pmatrix} 0 \\ 0 \\ 0 \end{pmatrix} & \begin{pmatrix} xxz \\ 0 \\ 0 \end{pmatrix} \\ \begin{pmatrix} 0 \\ 0 \\ 0 \end{pmatrix} & \begin{pmatrix} 0 \\ 0 \\ yyz \end{pmatrix} & \begin{pmatrix} 0 \\ yyz \\ 0 \end{pmatrix} \\ \begin{pmatrix} zxx \\ 0 \\ 0 \end{pmatrix} & \begin{pmatrix} 0 \\ zyy \\ 0 \end{pmatrix} & \begin{pmatrix} 0 \\ 0 \\ zzz \end{pmatrix} \end{pmatrix}$$

$$\boldsymbol{I^{PP}}(\boldsymbol{2\omega}) \sim \left(\chi_{zzz}\sin^3(\theta) + \sin(\theta)\cos^2(\theta)\left((-2\chi_{xxz} + \chi_{zxx})\,\mathbf{cos^2}(\boldsymbol{\varphi}) + \left(-2\chi_{yyz} + \chi_{zyy}\right)\mathbf{sin^2}(\boldsymbol{\varphi})\right)\right)^2$$

$$\boldsymbol{I^{PS}}(\boldsymbol{2\omega}) \sim 4\sin^2(\theta)\cos^2(\theta)\left(\left(\chi_{xxz} - \chi_{yyz}\right)\mathbf{sin}(\boldsymbol{\varphi})\mathbf{cos}(\boldsymbol{\varphi})\right)^2$$

$$\boldsymbol{I^{SP}}(\boldsymbol{2\omega}) \sim \sin^2(\theta)(\chi_{zxx}\,\mathbf{sin^2}(\boldsymbol{\varphi}) + \chi_{zyy}\,\mathbf{cos^2}(\boldsymbol{\varphi}))^2$$

$$\boldsymbol{I^{SS}}(\boldsymbol{2\omega}) = 0$$

*I3*,$\{\boldsymbol{4mm}\}$

$$\chi_{ijk}^{ED} = \begin{pmatrix} \begin{pmatrix} 0 \\ 0 \\ \mathrm{xxz} \end{pmatrix} & \begin{pmatrix} 0 \\ 0 \\ 0 \end{pmatrix} & \begin{pmatrix} \mathrm{xxz} \\ 0 \\ 0 \end{pmatrix} \\ \begin{pmatrix} 0 \\ 0 \\ 0 \end{pmatrix} & \begin{pmatrix} 0 \\ 0 \\ \mathrm{xxz} \end{pmatrix} & \begin{pmatrix} 0 \\ \mathrm{xxz} \\ 0 \end{pmatrix} \\ \begin{pmatrix} \mathrm{zxx} \\ 0 \\ 0 \end{pmatrix} & \begin{pmatrix} 0 \\ zxx \\ 0 \end{pmatrix} & \begin{pmatrix} 0 \\ 0 \\ \mathrm{zzz} \end{pmatrix} \end{pmatrix}$$

$$\boldsymbol{I^{PP}}(\boldsymbol{2\omega}) \sim \left[\sin^2(\theta)\left((-2\chi_{\mathrm{xxz}} + \chi_{\mathrm{zxx}})\cos^2(\theta) - \chi_{\mathrm{zzz}}\sin(\theta)\right)^2\right]$$

$$\boldsymbol{I^{PS}}(\boldsymbol{2\omega}) = 0$$

$$\boldsymbol{I^{SP}}(\boldsymbol{2\omega}) \sim [\chi_{\mathrm{zxx}}{}^2\sin^2(\theta)]$$

$$\boldsymbol{I^{SS}}(\boldsymbol{2\omega}) = 0$$

## MD tensors

*D3*, {$\boldsymbol{mmm1'}$}

$$\chi_{ijk}^{MD} = \begin{pmatrix} \begin{pmatrix} 0 \\ 0 \\ 0 \end{pmatrix} & \begin{pmatrix} 0 \\ 0 \\ \mathrm{xyz} \end{pmatrix} & \begin{pmatrix} 0 \\ \mathrm{xzy} \\ 0 \end{pmatrix} \\ \begin{pmatrix} 0 \\ 0 \\ \mathrm{yxz} \end{pmatrix} & \begin{pmatrix} 0 \\ 0 \\ 0 \end{pmatrix} & \begin{pmatrix} \mathrm{yzx} \\ 0 \\ 0 \end{pmatrix} \\ \begin{pmatrix} 0 \\ \mathrm{zxy} \\ 0 \end{pmatrix} & \begin{pmatrix} \mathrm{zyx} \\ 0 \\ 0 \end{pmatrix} & \begin{pmatrix} 0 \\ 0 \\ 0 \end{pmatrix} \end{pmatrix}$$

$$\boldsymbol{I^{PP}}(2\boldsymbol{\omega}) \sim \left[ \sin^2(2\theta) \left( (\chi_{\mathrm{xyz}} - \chi_{\mathrm{zyx}}) \mathbf{cos^2}(\boldsymbol{\varphi}) + (-\chi_{\mathrm{yxz}} + \chi_{\mathrm{zxy}}) \, \mathbf{sin^2}(\boldsymbol{\varphi}) \right)^2 \right]$$

$$\boldsymbol{I^{PS}}(\mathbf{2}\boldsymbol{\omega}) \sim \left[ (\chi_{\mathrm{xyz}} + \chi_{\mathrm{yxz}})^{\mathbf{2}} \mathbf{cos^2}(\boldsymbol{\varphi}) \, \mathbf{sin^2}(\boldsymbol{\varphi}) \sin^2(\theta) \right]$$

$$\boldsymbol{I^{SP}}(\mathbf{2}\boldsymbol{\omega}) \sim \left[ \left( (-\chi_{\mathrm{xyz}} + \chi_{\mathrm{zyx}}) \mathbf{cos^2}(\boldsymbol{\varphi}) + (\chi_{\mathrm{yxz}} - \chi_{\mathrm{zxy}}) \, \mathbf{sin^2}(\boldsymbol{\varphi}) \right)^2 \cos^2(\theta) \sin^2(\theta) \right]$$

$$\boldsymbol{I^{SS}}(\mathbf{2}\boldsymbol{\omega}) \sim \left[ (\chi_{\mathrm{xyz}} + \chi_{\mathrm{yxz}})^{\mathbf{2}} \mathbf{cos^2}(\boldsymbol{\varphi}) \, \mathbf{sin^2}(\boldsymbol{\varphi}) \sin^2(\theta) \right]$$

*F3*, {**4/*m***}

$$\chi_{ijk}^{MD} = \begin{pmatrix} \begin{pmatrix} 0 \\ 0 \\ \mathrm{xxz} \end{pmatrix} & \begin{pmatrix} 0 \\ 0 \\ \mathrm{xyz} \end{pmatrix} & \begin{pmatrix} \mathrm{xzx} \\ \mathrm{xzy} \\ 0 \end{pmatrix} \\ \begin{pmatrix} 0 \\ 0 \\ -\mathrm{xyz} \end{pmatrix} & \begin{pmatrix} 0 \\ 0 \\ \mathrm{xxz} \end{pmatrix} & \begin{pmatrix} -\mathrm{xzy} \\ \mathrm{xzx} \\ 0 \end{pmatrix} \\ \begin{pmatrix} \mathrm{zxx} \\ \mathrm{zxy} \\ 0 \end{pmatrix} & \begin{pmatrix} -\mathrm{zxy} \\ \mathrm{zxx} \\ 0 \end{pmatrix} & \begin{pmatrix} 0 \\ 0 \\ \mathrm{zzz} \end{pmatrix} \end{pmatrix}$$

$$\boldsymbol{I^{PP}}(2\boldsymbol{\omega}) \sim \left[ (\chi_{\mathrm{xyz}} - \chi_{\mathrm{zxy}})^2 \cos^2(\theta) \sin^2(\theta) \right]$$

$$\boldsymbol{I^{PS}}(\mathbf{2}\boldsymbol{\omega}) \sim [\chi_{\mathrm{xzx}} \sin^2(\theta)]$$

$$\boldsymbol{I^{SP}}(\mathbf{2}\boldsymbol{\omega}) \sim \left[ (\chi_{\mathrm{xyz}} + \chi_{\mathrm{zxy}})^2 \cos^2(\theta) \sin^2(\theta) \right]$$

$$\boldsymbol{I^{SS}}(\mathbf{2}\boldsymbol{\omega}) \sim [\chi_{\mathrm{xxz}} \sin^2(\theta)]$$

*H3*, {**4/mmm, 4/mm′m′ (*i*), 4′/mmm′ (*i*)**}

$$\chi_{ijk}^{MD} = \begin{pmatrix} \begin{pmatrix} 0 \\ 0 \\ 0 \end{pmatrix} & \begin{pmatrix} 0 \\ 0 \\ \mathrm{xyz} \end{pmatrix} & \begin{pmatrix} 0 \\ \mathrm{xyz} \\ 0 \end{pmatrix} \\ \begin{pmatrix} 0 \\ 0 \\ -\mathrm{xyz} \end{pmatrix} & \begin{pmatrix} 0 \\ 0 \\ 0 \end{pmatrix} & \begin{pmatrix} -\mathrm{xyz} \\ 0 \\ 0 \end{pmatrix} \\ \begin{pmatrix} 0 \\ \mathrm{zxy} \\ 0 \end{pmatrix} & \begin{pmatrix} -zxy \\ 0 \\ 0 \end{pmatrix} & \begin{pmatrix} 0 \\ 0 \\ 0 \end{pmatrix} \end{pmatrix}$$

$\boldsymbol{I^{PP}}(2\boldsymbol{\omega}) \sim \left[\left(\chi_{\mathrm{xyz}} - \chi_{\mathrm{zxy}}\right)^2 \cos^2(\theta)\sin^2(\theta)\right]$

$\boldsymbol{I^{PS}}(\boldsymbol{2\omega}) \sim 0$

$\boldsymbol{I^{SP}}(\boldsymbol{2\omega}) \sim \left[\left(\chi_{\mathrm{xyz}} + \chi_{\mathrm{zxy}}\right)^2 \cos^2(\theta)\sin^2(\theta)\right]$

$\boldsymbol{I^{SS}}(\boldsymbol{2\omega}) \sim 0$

*I3*, {**4/mm′m′ (*c*)**}

$$\chi_{ijk}^{MD} = \begin{pmatrix} \begin{pmatrix} 0 \\ 0 \\ \mathrm{xxz} \end{pmatrix} & \begin{pmatrix} 0 \\ 0 \\ 0 \end{pmatrix} & \begin{pmatrix} \mathrm{xzx} \\ 0 \\ 0 \end{pmatrix} \\ \begin{pmatrix} 0 \\ 0 \\ 0 \end{pmatrix} & \begin{pmatrix} 0 \\ 0 \\ \mathrm{xxz} \end{pmatrix} & \begin{pmatrix} 0 \\ \mathrm{xzx} \\ 0 \end{pmatrix} \\ \begin{pmatrix} \mathrm{zxx} \\ 0 \\ 0 \end{pmatrix} & \begin{pmatrix} 0 \\ zxx \\ 0 \end{pmatrix} & \begin{pmatrix} 0 \\ 0 \\ \mathrm{zzz} \end{pmatrix} \end{pmatrix}$$

$\boldsymbol{I^{PP}}(2\boldsymbol{\omega}) \sim 0$

$\boldsymbol{I^{PS}}(\boldsymbol{2\omega}) \sim [\chi_{\mathrm{xzx}}{}^2 \sin^2(\theta)]$

$\boldsymbol{I^{SP}}(\boldsymbol{2\omega}) \sim 0$

$\boldsymbol{I^{SS}}(\boldsymbol{2\omega}) \sim [\chi_{\mathrm{xxz}}{}^2 \sin^2(\theta)]$

*J3*, {**4′/mmm′(c)**}

$$\chi_{ijk}^{MD} = \begin{pmatrix} \begin{pmatrix} 0 \\ 0 \\ 0 \end{pmatrix} & \begin{pmatrix} 0 \\ 0 \\ \mathrm{xyz} \end{pmatrix} & \begin{pmatrix} 0 \\ \mathrm{xzy} \\ 0 \end{pmatrix} \\ \begin{pmatrix} 0 \\ 0 \\ \mathrm{xyz} \end{pmatrix} & \begin{pmatrix} 0 \\ 0 \\ 0 \end{pmatrix} & \begin{pmatrix} \mathrm{xzy} \\ 0 \\ 0 \end{pmatrix} \\ \begin{pmatrix} 0 \\ \mathrm{zx}y \\ 0 \end{pmatrix} & \begin{pmatrix} zxy \\ 0 \\ 0 \end{pmatrix} & \begin{pmatrix} 0 \\ 0 \\ 0 \end{pmatrix} \end{pmatrix}$$

$$\boldsymbol{I^{PP}}(2\boldsymbol{\omega}) \sim \left[\left(\chi_{\mathrm{xyz}} - \chi_{\mathrm{zxy}}\right)^2 \mathbf{cos^2}(\mathbf{2}\boldsymbol{\varphi}) \sin^2(2\theta)\right]$$

$$\boldsymbol{I^{PS}}(\mathbf{2}\boldsymbol{\omega}) \sim \left[\left(\chi_{\mathrm{xzy}}\right)^2 \cos^2(\theta) \, \mathbf{sin^2}(\mathbf{2}\boldsymbol{\varphi})\right]$$

$$\boldsymbol{I^{SP}}(\mathbf{2}\boldsymbol{\omega}) \sim \left[\left(\chi_{\mathrm{xyz}} - \chi_{\mathrm{zxy}}\right)^2 \mathbf{cos^2}(\mathbf{2}\boldsymbol{\varphi}) \sin^2(2\theta)\right]$$

$$\boldsymbol{I^{SS}}(\mathbf{2}\boldsymbol{\omega}) \sim \left[\left(\chi_{\mathrm{xyz}}\right)^2 \cos^2(\theta) \, \mathbf{sin^2}(\mathbf{2}\boldsymbol{\varphi})\right]$$

## EQ tensors

*D4*, $\{\boldsymbol{mmm1'}\}$

$$\chi^{EQ}_{ijkl} = \begin{pmatrix} \begin{pmatrix} xxxx & 0 & 0 \\ 0 & xxyy & 0 \\ 0 & 0 & xxzz \end{pmatrix} & \begin{pmatrix} 0 & xyxy & 0 \\ xxyy & 0 & 0 \\ 0 & 0 & 0 \end{pmatrix} & \begin{pmatrix} 0 & 0 & xzxz \\ 0 & 0 & 0 \\ xxzz & 0 & 0 \end{pmatrix} \\ \begin{pmatrix} 0 & yxxy & 0 \\ yxyx & 0 & 0 \\ 0 & 0 & 0 \end{pmatrix} & \begin{pmatrix} yyxx & 0 & 0 \\ 0 & yyyy & 0 \\ 0 & 0 & yyzz \end{pmatrix} & \begin{pmatrix} 0 & 0 & 0 \\ 0 & 0 & yzyz \\ 0 & yyzz & 0 \end{pmatrix} \\ \begin{pmatrix} 0 & 0 & zzxx \\ 0 & 0 & 0 \\ zxzx & 0 & 0 \end{pmatrix} & \begin{pmatrix} 0 & 0 & 0 \\ 0 & 0 & zzyy \\ 0 & zyzy & 0 \end{pmatrix} & \begin{pmatrix} zzxx & 0 & 0 \\ 0 & zzyy & 0 \\ 0 & 0 & zzzz \end{pmatrix} \end{pmatrix}$$

$$\begin{aligned} \boldsymbol{I^{PP}(2\omega)} \sim \Big[&\cos(\theta)\sin^3(\theta)\left(\chi_{zzzz} + (\chi_{xzxz} - 2\chi_{zzxx})\,\mathbf{cos^2}(\boldsymbol{\varphi}) + \left(\chi_{yzyz} - 2\chi_{zzyy}\right)\mathbf{sin^2}(\boldsymbol{\varphi})\right) \\ &- \sin(\theta)\cos^3(\theta)\,(-\chi_{xxxx}\,\mathbf{cos^4}(\boldsymbol{\varphi}) \\ &+ \big(2\chi_{xxzz} - \chi_{zxzx} \\ &- \left(2\chi_{xxyy} + \chi_{xyxy} + \chi_{yxxy} + \chi_{yxyx} + \chi_{yyxx}\right)\mathbf{sin^2}(\boldsymbol{\varphi})\big)\,\mathbf{cos^2}(\boldsymbol{\varphi}) \\ &- \mathbf{sin^2}(\boldsymbol{\varphi})\,(-2\chi_{yyzz} + \chi_{zyzy} + \chi_{yyyy}\,\mathbf{sin^2}(\boldsymbol{\varphi})))^2\Big] \end{aligned}$$

$$\begin{aligned} \boldsymbol{I^{PS}(2\omega)} \sim \Bigg[&\sin(\theta)\Big(\left(-\chi_{xzxz} + \chi_{yzyz}\right)\sin^2(\theta)\,\mathbf{cos}(\boldsymbol{\varphi})\,\mathbf{sin}(\boldsymbol{\varphi}) \\ &+ \cos^2(\theta)\Big(\left(-\chi_{xxxx} + \chi_{yxxy} + \chi_{xyxy} + \chi_{yyxx}\right)\mathbf{cos^3}(\boldsymbol{\varphi})\,\mathbf{sin}(\boldsymbol{\varphi}) - (2\chi_{xxyy} \\ &+ \chi_{xyxy} - \chi_{yyyy})\,\mathbf{cos}(\boldsymbol{\varphi})\,\mathbf{sin^3}(\boldsymbol{\varphi}) + \left(\chi_{xxzz} - \chi_{yyzz}\right)\mathbf{sin}(\mathbf{2}\boldsymbol{\varphi})\Big)\Big)^2\Bigg] \end{aligned}$$

$$\begin{aligned} \boldsymbol{I^{SP}(2\omega)} \sim \Big[&\cos^2(\theta)\sin^2(\theta)\Big(\big(\chi_{xyxy}\,\mathbf{cos^4}(\boldsymbol{\varphi}) + \chi_{yxyx}\,\mathbf{sin^4}(\boldsymbol{\varphi}) \\ &+ \left(\chi_{xxxx} - 2\chi_{xxyy} - \chi_{yxxy} - \chi_{yyxx} + \chi_{yyyy}\right)\mathbf{cos^2}(\boldsymbol{\varphi})\,\mathbf{sin^2}(\boldsymbol{\varphi})\big) \\ &+ \left(\chi_{zyzy}\,\mathbf{cos^2}(\boldsymbol{\varphi}) + \chi_{zxzx}\,\mathbf{sin^2}(\boldsymbol{\varphi})\right)\Big)^2\Big] \end{aligned}$$

$$\begin{aligned} \boldsymbol{I^{SS}(2\omega)} \sim \Big[&\Big(\left(\chi_{xxxx} - 2\chi_{xxyy} - \chi_{yxyx}\right)\mathbf{sin^2}(\boldsymbol{\varphi}) \\ &+ \left(\chi_{xxxx} + \chi_{yyxx} + \chi_{yyxx} + \chi_{yyyy}\right)\mathbf{cos^2}(\boldsymbol{\varphi})\Big)^2\sin^2(\theta)\,\mathbf{cos^2}(\boldsymbol{\varphi})\,\mathbf{sin^2}(\boldsymbol{\varphi})\Big] \end{aligned}$$

*F4*, {**4/m**}

$$\chi_{ijkl}^{EQ} = \begin{pmatrix} \begin{pmatrix} \text{xxxx} & \text{xxxy} & 0 \\ \text{xxyx} & \text{xxyy} & 0 \\ 0 & 0 & \text{xxzz} \end{pmatrix} & \begin{pmatrix} \text{xxxy} & \text{xyxy} & 0 \\ \text{xxyy} & \text{xyyy} & 0 \\ 0 & 0 & \text{xyzz} \end{pmatrix} & \begin{pmatrix} 0 & 0 & \text{xzxz} \\ 0 & 0 & \text{xzyz} \\ \text{xxzz} & \text{xyzz} & 0 \end{pmatrix} \\ \begin{pmatrix} -\text{xyyy} & \text{xxyy} & 0 \\ \text{xyxy} & -\text{xxxy} & 0 \\ 0 & 0 & -\text{xyzz} \end{pmatrix} & \begin{pmatrix} \text{xxyy} & -\text{xxyx} & 0 \\ -\text{xxxy} & \text{xxxx} & 0 \\ 0 & 0 & \text{xxzzx} \end{pmatrix} & \begin{pmatrix} 0 & 0 & -\text{xzyz} \\ 0 & 0 & \text{xzxz} \\ -\text{xyzz} & \text{xxzz} & 0 \end{pmatrix} \\ \begin{pmatrix} 0 & 0 & \text{zzxx} \\ 0 & 0 & \text{zxyz} \\ \text{zxzx} & 0 & 0 \end{pmatrix} & \begin{pmatrix} 0 & 0 & -\text{zxyz} \\ 0 & 0 & \text{zzxx} \\ 0 & \text{zxzx} & 0 \end{pmatrix} & \begin{pmatrix} \text{zzxx} & \text{zzxy} & 0 \\ -\text{zzxy} & \text{zzxx} & 0 \\ 0 & 0 & \text{zzzz} \end{pmatrix} \end{pmatrix}$$

$$\boldsymbol{I^{PP}(2\omega)} \sim \Big[\big(4(\chi_{zzzz} - 2\chi_{zzxx} + \chi_{xzxz})\cos(\theta)\sin^3(\theta) + \sin(\theta)\cos^3(\theta)\big(3\chi_{xxxx} + 2\chi_{xxyy} - 8\chi_{xxzz} + \chi_{xyxy} + 4\chi_{zxzx} + (\chi_{xxxx} - 2\chi_{xxyy} - \chi_{xyxy})\,\mathbf{cos(4\boldsymbol{\varphi})} - (2\chi_{xxxy} - \chi_{xxyx} + \chi_{xyyy})\,\mathbf{sin(4\boldsymbol{\varphi})}\big)\big)^2\Big]$$

$$\boldsymbol{I^{PS}(2\omega)} \sim \Big[\Big(4\chi_{zzxy}\sin^3(\theta) + \cos^2(\theta)\sin(\theta)\big(2\chi_{xxxy} + \chi_{xxyx} + 3\chi_{xxyx} - 8\chi_{xyzz} + (-2\chi_{xxxy} - \chi_{xxyx} + \chi_{xyyy})\,\mathbf{cos(4\boldsymbol{\varphi})} + (-\chi_{xxxx} + 2\chi_{xxxy} + \chi_{xyxy})\,\mathbf{sin(4\boldsymbol{\varphi})}\big)\Big)^2\Big]$$

$$\boldsymbol{I^{SP}(2\omega)} \sim \Bigg[\Bigg(-\chi_{zxzx}\cos(\theta)\sin(\theta) - \frac{1}{4}\cos(\theta)\sin(\theta)\big(\chi_{xxxx} - 2\chi_{xxyy} + 3\chi_{xyxy} - (\chi_{xxxx} - 2\chi_{xxyy} - \chi_{xyxy})\,\mathbf{cos(4\boldsymbol{\varphi})} + (2\chi_{xxxy} + \chi_{xxyx} - \chi_{xyyy})\,\mathbf{sin(4\boldsymbol{\varphi})}\big)\Bigg)^2\Bigg]$$

$$\boldsymbol{I^{SS}(2\omega)} \sim \Big[\sin^2(\theta)\big(-2\chi_{xxxy} + 3\chi_{xxyx} + \chi_{xyyy} + (2\chi_{xxxy} + \chi_{xxyx} - \chi_{xyyy})\,\mathbf{cos(4\boldsymbol{\varphi})} + (\chi_{xxxx} - 2\chi_{xxyy} - \chi_{xyxy})\,\mathbf{sin(4\boldsymbol{\varphi})}\big)^2\Big]$$

*H4*, {**4/*mmm*, 4*mm*, 4/*mm*′*m*′ (*i*), 4′/*mmm*′ (*i*)**}

$$\chi_{ijkl}^{EQ} = \begin{pmatrix} \begin{pmatrix} xxxx & 0 & 0 \\ 0 & xxyy & 0 \\ 0 & 0 & xxzz \end{pmatrix} & \begin{pmatrix} 0 & xyxy & 0 \\ xxyy & 0 & 0 \\ 0 & 0 & 0 \end{pmatrix} & \begin{pmatrix} 0 & 0 & xzxz \\ 0 & 0 & 0 \\ xxzz & 0 & 0 \end{pmatrix} \\ \begin{pmatrix} 0 & xxyy & 0 \\ xyxy & 0 & 0 \\ 0 & 0 & 0 \end{pmatrix} & \begin{pmatrix} xxyy & 0 & 0 \\ 0 & xxxx & 0 \\ 0 & 0 & xxzz \end{pmatrix} & \begin{pmatrix} 0 & 0 & 0 \\ 0 & 0 & xzxz \\ 0 & xxzz & 0 \end{pmatrix} \\ \begin{pmatrix} 0 & 0 & zzxx \\ 0 & 0 & 0 \\ zxzx & 0 & 0 \end{pmatrix} & \begin{pmatrix} 0 & 0 & 0 \\ 0 & 0 & zzxx \\ 0 & zxzx & 0 \end{pmatrix} & \begin{pmatrix} zzxx & 0 & 0 \\ 0 & zzxx & 0 \\ 0 & 0 & zzzz \end{pmatrix} \end{pmatrix}$$

$$\boldsymbol{I^{PP}(2\omega)} \sim \left[\left(\cos^3(\theta)\sin(\theta)\left(3\chi_{xxxx} + 2\chi_{xxyy} - 8\chi_{xxzz} + \chi_{xyxy} + 4\chi_{zxzx} + \left(\chi_{xxxx} - 2\chi_{xxyy} - \chi_{xyxy}\right)\boldsymbol{\cos(4\varphi)}\right) + 4(-2\chi_{zzxx} + \chi_{zzzz} + \chi_{xzxz})\sin^3(\theta)\cos(\theta)\right)^2\right]$$

$$\boldsymbol{I^{PS}(2\omega)} \sim \left[\left(-\chi_{xxxx} + 2\chi_{xxyy} + \chi_{xyxy}\right)^2 \cos^4(\theta)\sin^2(\theta)\,\boldsymbol{\sin^2(4\varphi)}\right]$$

$$\boldsymbol{I^{SP}(2\omega)} \sim \left[\left(-\chi_{zxzx}\cos(\theta)\sin(\theta) + \frac{1}{4}\cos(\theta)\left(\chi_{xxxx} - 2\chi_{xxyy} + 3\chi_{xyxy} + (-\chi_{xxxx} + 2\chi_{xxyy} + \chi_{xyxy})\,\boldsymbol{\cos(4\varphi)}\right)\right)^2 \sin^2(\theta)\right]$$

$$\boldsymbol{I^{SS}(2\omega)} \sim \left[\left(-\chi_{xxxx} + 2\chi_{xxyy} + \chi_{xyxy}\right)^2 \sin^2(\theta)\,\boldsymbol{\sin^2(4\varphi)}\right]$$

*I*4, {**4/*mm*′*m*′ (*c*)**}

$$\chi_{ijkl}^{EQ} = \begin{pmatrix} \begin{pmatrix} 0 & \mathrm{xxxy} & 0 \\ \mathrm{xxyx} & 0 & 0 \\ 0 & 0 & 0 \end{pmatrix} & \begin{pmatrix} \mathrm{xxxy} & 0 & 0 \\ 0 & \mathrm{xyyy} & 0 \\ 0 & 0 & \mathrm{zzxy} \end{pmatrix} & \begin{pmatrix} 0 & 0 & 0 \\ 0 & 0 & \mathrm{zzxy} \\ 0 & \mathrm{zzxy} & 0 \end{pmatrix} \\ \begin{pmatrix} -\mathrm{xyyy} & 0 & 0 \\ 0 & -\mathrm{xxxy} & 0 \\ 0 & 0 & -\mathrm{xyzz} \end{pmatrix} & \begin{pmatrix} 0 & -\mathrm{xxyx} & 0 \\ -\mathrm{xxxy} & 0 & 0 \\ 0 & 0 & 0 \end{pmatrix} & \begin{pmatrix} 0 & 0 & -\mathrm{xzyz} \\ 0 & 0 & 0 \\ -\mathrm{xyzz} & 0 & 0 \end{pmatrix} \\ \begin{pmatrix} 0 & 0 & 0 \\ 0 & 0 & \mathrm{zxyz} \\ 0 & 0 & 0 \end{pmatrix} & \begin{pmatrix} 0 & 0 & -\mathrm{zxyz} \\ 0 & 0 & 0 \\ 0 & 0 & 0 \end{pmatrix} & \begin{pmatrix} 0 & \mathrm{zzxy} & 0 \\ -\mathrm{zzxy} & 0 & 0 \\ 0 & 0 & 0 \end{pmatrix} \end{pmatrix}$$

$$\boldsymbol{I^{PP}}(2\boldsymbol{\omega}) \sim \left[\left(2\chi_{\mathrm{xxxy}} + \chi_{\mathrm{xxyx}} - \chi_{\mathrm{xyyy}}\right)^2 \cos^6(\theta)\sin^2(\theta)\,\mathbf{sin^2}(\mathbf{4}\boldsymbol{\varphi})\right]$$

$$\boldsymbol{I^{PS}}(\mathbf{2}\boldsymbol{\omega}) \sim \Big[\sin^2(\theta)\left(\cos^2(\theta)\left(2\chi_{\mathrm{xxxy}} + \chi_{\mathrm{xxyx}} - 8\chi_{\mathrm{xyzz}} + 3\chi_{\mathrm{xyyy}} + \left(-2\chi_{\mathrm{xxxy}} - \chi_{\mathrm{xxyx}} + \chi_{\mathrm{xyyy}}\right)\mathbf{cos}(\mathbf{4}\boldsymbol{\varphi})]\right) + 4\chi_{\mathrm{xzyz}}\sin^2(\theta)\right)^2\Big]$$

$$\boldsymbol{I^{SP}}(\mathbf{2}\boldsymbol{\omega}) \sim \left[\left(2\chi_{\mathrm{xxxy}} + \chi_{\mathrm{xxyx}} - \chi_{\mathrm{xyyy}}\right)^2 \cos^2(\theta)\sin^2(\theta)\,\mathbf{sin^2}(\mathbf{4}\boldsymbol{\varphi})\right]$$

$$\boldsymbol{I^{SS}}(\mathbf{2}\boldsymbol{\omega}) \sim \left[\left(-2\chi_{\mathrm{xxxy}} + 3\chi_{\mathrm{xxyx}} + \chi_{\mathrm{xyyy}} + \left(2\chi_{\mathrm{xxxy}} + \chi_{\mathrm{xxyx}} - \chi_{\mathrm{xyyy}}\right)\mathbf{cos}(\mathbf{4}\boldsymbol{\varphi})\right)^2 \sin^2(\theta)\right]$$

*J4*, {**4′/mmm′ (c)**}

$$\chi_{ijkl}^{EQ} = \begin{pmatrix} \begin{pmatrix} \mathrm{xxxx} & 0 & 0 \\ 0 & \mathrm{xxyy} & 0 \\ 0 & 0 & \mathrm{xxzz} \end{pmatrix} & \begin{pmatrix} 0 & \mathrm{xyxy} & 0 \\ \mathrm{xxyy} & 0 & 0 \\ 0 & 0 & 0 \end{pmatrix} & \begin{pmatrix} 0 & 0 & \mathrm{xzxz} \\ 0 & 0 & 0 \\ \mathrm{xxzz} & 0 & 0 \end{pmatrix} \\ \begin{pmatrix} 0 & -\mathrm{xxyy} & 0 \\ -\mathrm{xyxy} & 0 & 0 \\ 0 & 0 & 0 \end{pmatrix} & \begin{pmatrix} -\mathrm{xxyy} & 0 & 0 \\ 0 & -\mathrm{xxxx} & 0 \\ 0 & 0 & -\mathrm{xxzz} \end{pmatrix} & \begin{pmatrix} 0 & 0 & 0 \\ 0 & 0 & -\mathrm{xzxz} \\ 0 & -\mathrm{xxzz} & 0 \end{pmatrix} \\ \begin{pmatrix} 0 & 0 & \mathrm{zzxx} \\ 0 & 0 & 0 \\ \mathrm{zxzx} & 0 & 0 \end{pmatrix} & \begin{pmatrix} 0 & 0 & 0 \\ 0 & 0 & -\mathrm{zzxx} \\ 0 & -\mathrm{zxzx} & 0 \end{pmatrix} & \begin{pmatrix} \mathrm{zzxx} & 0 & 0 \\ 0 & \mathrm{zzyy} & 0 \\ 0 & 0 & 0 \end{pmatrix} \end{pmatrix}$$

$$\boldsymbol{I^{PP}}(\mathbf{2}\boldsymbol{\omega}) \sim \left[\cos(\theta)\sin^3(\theta)\left(\chi_{zzxx}+\chi_{zzyy} - \left(2\chi_{xzxz} - 3\chi_{zzxx}+\chi_{zzyy}\right)\mathbf{cos^2}(\boldsymbol{\varphi})\right) - \sin(\theta)\cos^3(\theta)\left(\chi_{xxxx} - 2\chi_{xxzz} + \chi_{zxzx}\right)\mathbf{cos^2}(\boldsymbol{\varphi})\right]$$

$$\boldsymbol{I^{PS}}(\mathbf{2}\boldsymbol{\omega}) \sim \left[\left(\left(\chi_{xxxx} + 2\chi_{xxyy} - 4\chi_{xyxy} + \chi_{xyxy}\right)\sin(\theta)\cos^2(\theta)\,\mathbf{cos}(\boldsymbol{\varphi})\,\mathbf{sin}(\boldsymbol{\varphi}) + \chi_{xzxz}\sin^3(\theta)\,\mathbf{sin}(\mathbf{2}\boldsymbol{\varphi})\right)^2\right]$$

$$\boldsymbol{I^{SP}}(\mathbf{2}\boldsymbol{\omega}) \sim \left[\cos^2(\theta)\sin^2(\theta)\left(\left(-\chi_{xyxy} + \chi_{zxzx}\right)\mathbf{cos}(\mathbf{2}\boldsymbol{\varphi})\right)^2\right]$$

$$\boldsymbol{I^{SS}}(\mathbf{2}\boldsymbol{\omega}) \sim \left[\left(\chi_{xxxx} - 2\chi_{xxyy} + \chi_{xyxy}\right)^2\sin^2(\theta)\,\mathbf{cos^2}(\boldsymbol{\varphi})\,\mathbf{sin^2}(\boldsymbol{\varphi})\right]$$

## 2. Comparison to GaAs

To quantify the SHG intensity from $Sr_2CuO_2Cl_2$, we perform measurements on GaAs – an inversion broken crystal often used as an SHG standard – under identical experimental conditions. As shown Figure S1, the RA-SHG intensity from $Sr_2CuO_2Cl_2$ is approximately $10^4$ times smaller than that of GaAs (001).

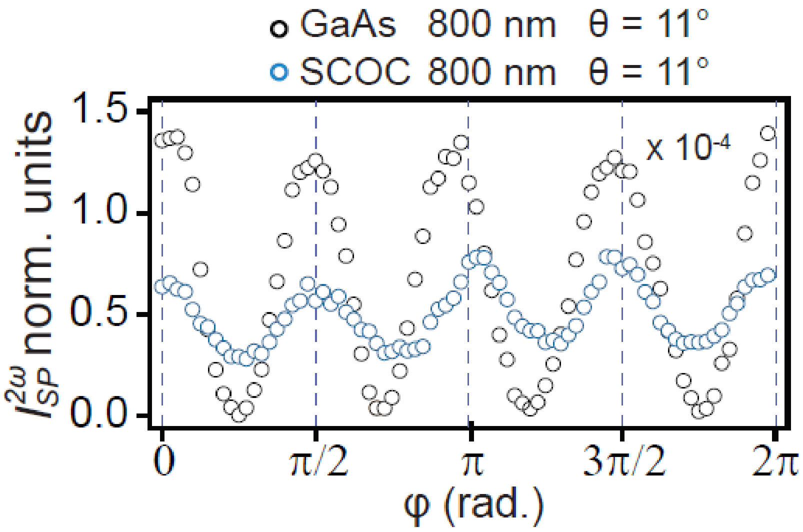


Figure S1: RA-SHG data from $Sr_2CuO_2Cl_2$ and GaAs (scaled by $10^{-4}$) measured at $T$ = 300 K in the SP channel under identical experimental conditions.

## 3. Simulated RA-SHG patterns using AFM point group

Figure S2 shows simulated RA-SHG patterns due to interference between an MD or EQ process from the magnetic point group *mmm*1′ and an EQ process from the crystallographic point group 4/*mmm*. As expected, the resulting RA-SHG patterns break $C_4$ as well as the *ac* and *bc* mirror planes but preserve the *xz* and *yz* mirror planes, making them incompatible with our data.

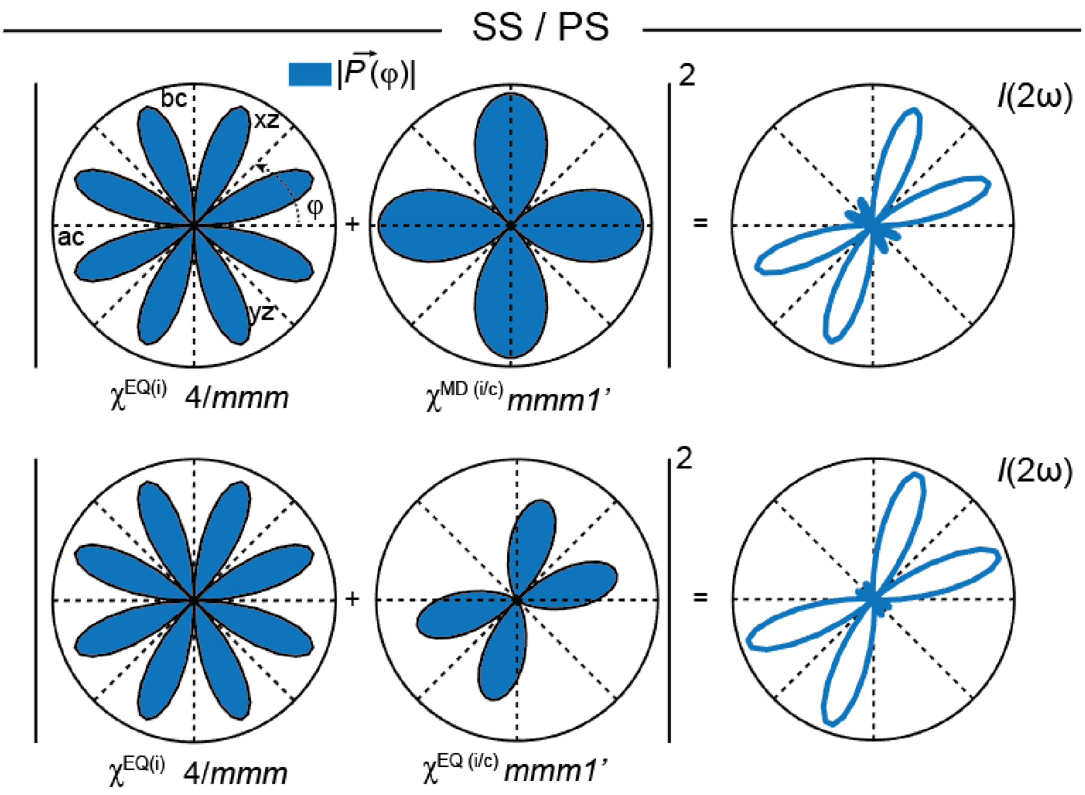


Figure S2: Simulated RA-SHG patterns assuming constructive interference between EQ SHG from 4/*mmm* and (top) MD or (bottom) EQ SHG from *mmm*1′. An arbitrary set of susceptibility tensor element values were used. These simulations are representative of both the PS and SS channels.

## 4. Description of possible $A_{2g}$ order parameters

As discussed in the main text, the order parameter associated with the $4/mm'm'$ magnetic point group has $A_{2g}$ symmetry. The simplest state that realizes this symmetry is a ferromagnet with a moment along *c*. But, as mentioned in the main text, canting has been ruled out by XMCD and is also inconsistent with $I4/mmm$, which does not allow for a DM interaction. On the other hand, magneto-chiral phases with this symmetry do exist, and are equivalent to an orbital ferromagnet with moment along *c* [Fig. S3(a)]. We note that below $T_N$, the actual magnetic point group of $Sr_2CuO_2Cl_2$ would be $mm'm'$, which is the intersection of $mmm1'$ with $4/mm'm'$.

In general, any axial harmonic with odd $L$ and $M = 0$ has $A_{2g}$ symmetry. An example is the (3,0) component of a magnetic octupole, which is illustrated in Figure S3(b). While we do not make any claims about its microscopic origin, we note that a ferroic ordering of (3,0) magnetic octupoles would be difficult to detect by more conventional methods like neutron or x-ray diffraction.

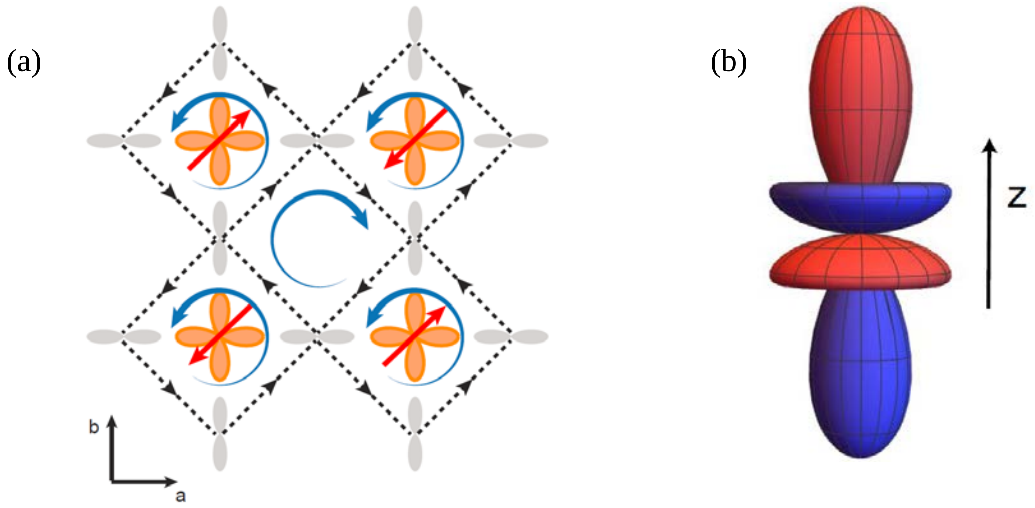


Figure S3: (a) Magneto-chiral loop current phase (dashed black arrows) superimposed on the AFM state (red arrows). The blue arrows schematically show the direction of orbital currents. Orange (gray) lobes denote the copper (oxygen) orbitals. (b) Schematic of the (3,0) component of a magnetic octupole. Red and blue encode opposite phase.

## 5. Temperature dependence of normal incidence intensity

Figure S4 shows the temperature dependence of the normal incidence SHG response of $Sr_2CuO_2Cl_2$ in both parallel (X-X) and perpendicular (X-Y) polarization channels. No discernible SHG signal is observed at any temperature.

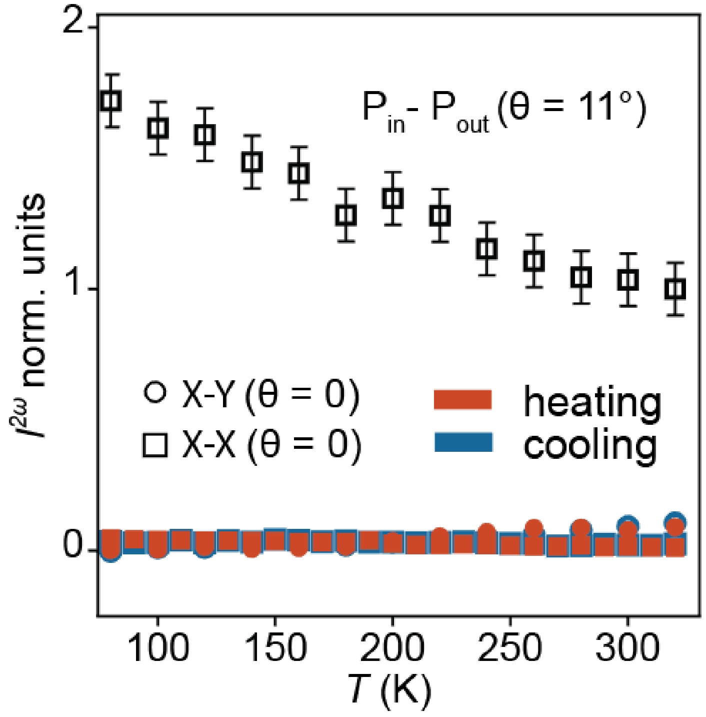


Figure S4: Temperature dependence of normal incidence SHG intensity for X-X and X-Y polarization channels measured using 800 nm light. The oblique incidence ($\theta = 11°$) SHG intensity measured in the PP channel with 800 nm light at $\varphi = \pi/4$ is shown for comparison. All data are normalized to the room temperature value of the PP curve.

## 6. Temperature dependence of intensity in PS and PP channels

Figure S5 shows the SHG intensity versus temperature in the PS and PP channels. It confirms that the feature at $T_N$ is only clearly observable in the S-output channels.

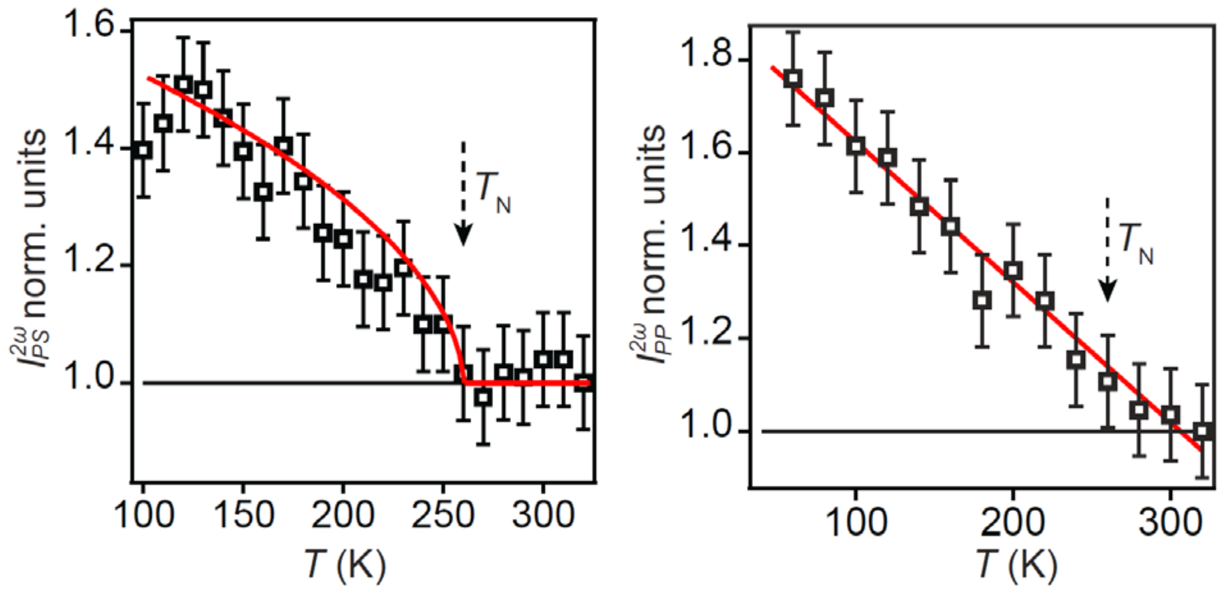


Figure S5: SHG intensity measured in the PS (φ = 3π/8) and PP (φ = π/4) channels at normalized to their $T$ = 320 K values. Red lines are guides to the eye.

## 7. Temperature and φ-dependence of intensity in SP and PP channels

To confirm that the lack of any feature at $T_N$ in the P-output channels is true at any φ, we collected full RA-SHG patterns as a function of temperature. As shown in Figure S6, no abrupt change of intensity or symmetry is observed near $T_N$ at all φ.

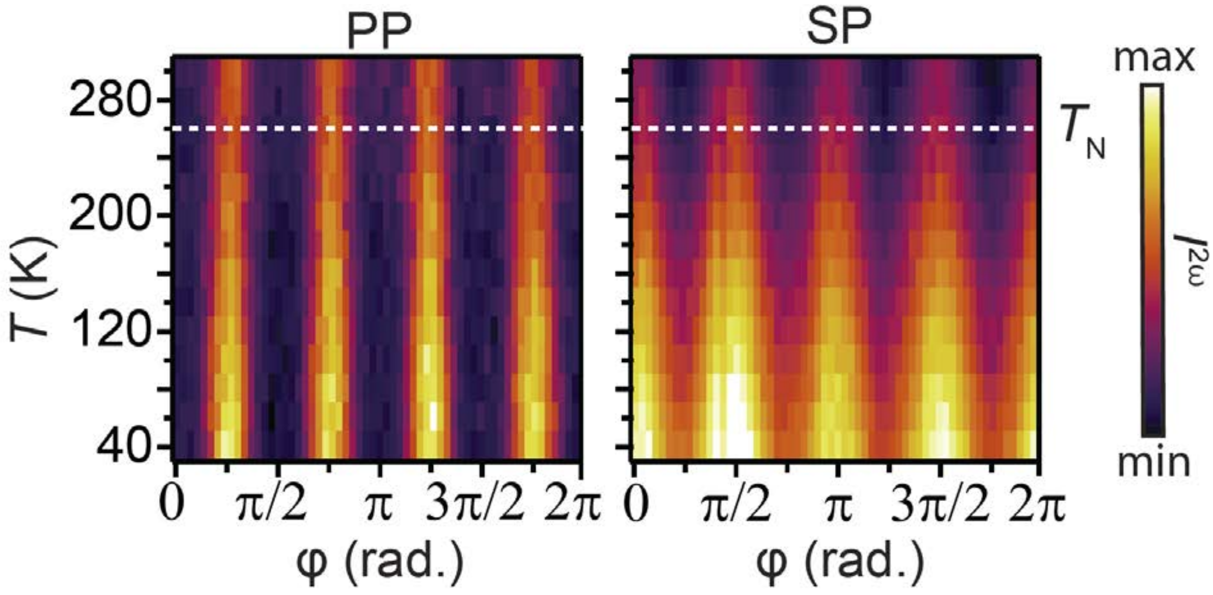


Figure S6: Temperature dependence of RA-SHG patterns in the P-output channels.

## 8. Effects of non-uniform lattice contraction

A non-uniform contraction of the *a* and *c* lattice constants of $Sr_2CuO_2Cl_2$ has been reported by neutron diffraction[3] and is shown in Figure S7(a). This change in lattice constants will change the relative magnitudes of the 4/*mmm* allowed crystallographic EQ SHG tensor elements. The significantly larger fractional contraction along the *c*-axis should lead to a stronger temperature dependence of the $\chi_{ijkl}^{EQ(i)}$ tensor elements with *i*, *j* or *l* = *z*, which only appear in the P-output channels. As a check, we fit the *T* = 320 K and *T* = 20 K data collected in the P-output channels to the function $(a + b\cos 4\varphi)^2$. As shown in section 1, $b = \left(\chi_{xxxx} - 2\chi_{xxyy} - \chi_{xyxy}\right)$ while the aforementioned *z* containing $\chi_{ijkl}^{EQ(i)}$ elements are all included in $a$. We first fit the *T* = 320 K data and obtained the following fit values. PP: (*a* = 0.71, *b* = -0.24), SP: (*a* = 0.95, *b* = 0.18). We then fit the *T* = 20 K data by keeping the *b*'s fixed to their high temperature values and letting only the *a*'s be free parameters. We obtained PP (*a* = 0.89, *b* = -0.24), SP (*a* = 1.60, *b* = 0.18). As shown in Figure S7(b), the temperature dependence of the RA-SHG patterns is very well captured by only changing the *a* terms. Allowing *a* to be complex does not change the conclusions.

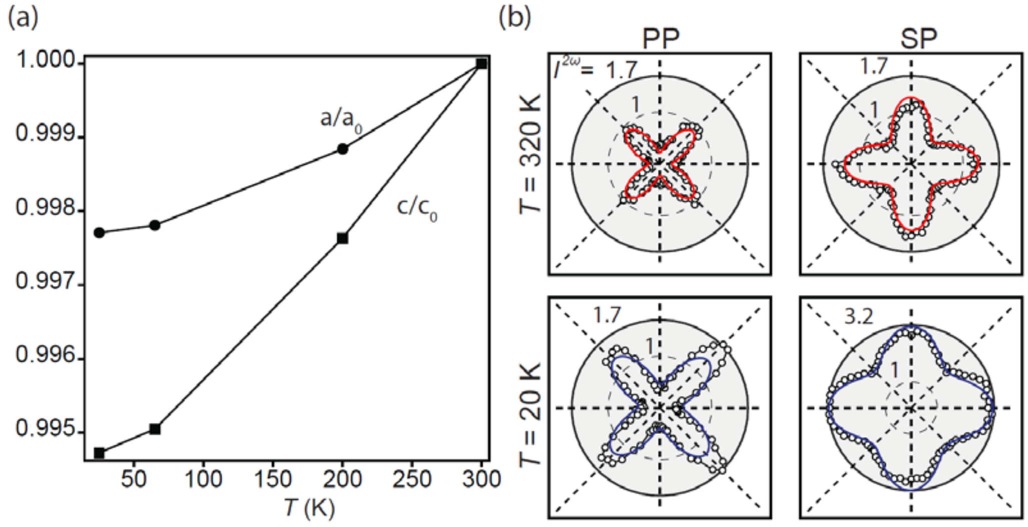


Figure S7: (a) Temperature dependence of the lattice parameters of $Sr_2CuO_2Cl_2$ reported by neutron diffraction[3]. (b) Fits (red/blue lines) to the RA-SHG data (circles/black lines) in the P-output channels. Fits to the *T* = 20 K data were obtained by allowing only *a* to vary and leaving *b* fixed to its *T* = 320 K value.

## 9. Laser fluence and average power considerations

As discussed in the Methods section, a minimum laser fluence of around 3 mJ/cm$^2$ at 1.5 eV photon energy was necessary to acquire RA-SHG patterns (especially in the SS channel) of reasonable quality. Based on prior time-resolved optical reflectivity measurements on $Sr_2CuO_2Cl_2$[4], no evidence of optical saturation is reported at this fluence level even at 3 eV photon energy, where the absorption is much higher than at 1.5 eV.

We estimate an upper limit to the steady state temperature increase of the sample ($\Delta T$) using the formula for the average heating of a Gaussian beam $\Delta T = \sqrt{\frac{\ln 2}{\pi}}\left(\frac{P}{\kappa l}\right)$. Here $P$ is the average laser power, $\kappa$ is the thermal conductivity and $l$ is the FWHM of our Gaussian beam spot. To achieve a fluence of 3 mJ/cm$^2$ we use $P$ = 3 mW and $l$ = 40 μm. Plugging in the reported in-plane value for the thermal conductivity[5] at 260 K ($\kappa$ = 10 W/K.m) we obtain $\Delta T$ = 3.5 K. This is consistent with the negligible difference between the value of $T_N$ observed in our SHG experiment and that reported in the literature.

## 10. Effects of thermal cycling

In attempt to stabilize a region with a time-reversed order parameter ($-\Phi$), we collected RA-SHG data in the SS channel from the same spots on $Sr_2CuO_2Cl_2$ under repeated thermal cycles across $T_N$. As shown in Figure S8, upon thermal cycling, the relative magnitude of adjacent lobes at low temperature does not change. This means that the sign of $\Phi$ does not flip.

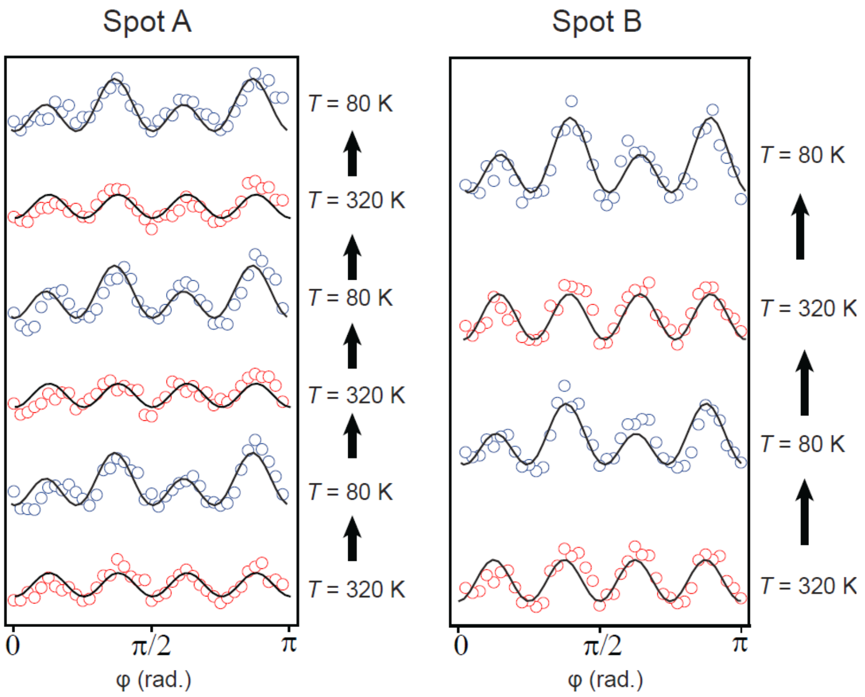


Figure S8: RA-SHG data in the SS channel measured from the same spot on $Sr_2CuO_2Cl_2$ upon successive thermal cycles at two different locations. Curves are vertically offset for clarity. Lines are guides to the eye.

## 11. Discussion of the effects of crystal imperfections

We discuss several types of possible imperfections in the crystallographic and magnetic structures of $Sr_2CuO_2Cl_2$ and their possible influence on the SHG response.

(1) While the average structure of $Sr_2CuO_2Cl_2$ is known to have a 4/*mmm* point group, it is possible that the local structure has lower symmetry. This can lead to a finite local spin canting even though it is forbidden in the average structure. Below we present several reasons why we can exclude local distortions, either dynamic or static, as the source of our SHG signal.

Consider dynamical fluctuations that generate a finite instantaneous spin canting, which time-averages to zero. Since our experiments average over many optical pulses, we are measuring a time-average over all instantaneous spin configurations, yielding no net symmetry breaking.

Next consider local static distortions that cause local static spin canting (either up or down), which averages to zero over space. If the characteristic structural modulation wavelength is much shorter than our optical wavelength (800 nm), then the SHG contributions from up and down regions add coherently, canceling out any spin-dependent contribution to SHG. If the modulation wavelength is longer than our optical wavelength, then the SHG contributions from up and down regions add incoherently, averaging away any symmetry reduction in the RA patterns.

(2) It is likely there are edge and/or screw dislocations in $Sr_2CuO_2Cl_2$ as a result of the crystal growth. This can lead to local crystallographic and spin structures that are different than the bulk. Below we outline reasons why such effects do not explain the SHG data. First, the new SHG contribution below $T_N$ is the same order of magnitude as the coherent EQ contribution above $T_N$. It is difficult to justify how a sparse density of dislocations and/or magnetic texture defects can generate such a large signal. Second, SHG from random scattering centers, either structural or magnetic, would be diffuse (hyper-Rayleigh) in nature[6]. But our SHG signal is highly specular, with no evidence of an increasing diffuse contribution below $T_N$. Third, dislocations and their induced magnetic texture defects would be expected to break the tetragonal symmetry of the average structure. This is hard to reconcile with the relatively high $4/mm'm'$ symmetry observed.

## 12. Comparison to prior SHG work on YBCO

Previous RA-SHG measurements on doped $YBa_2Cu_3O_y$ revealed a loss of vertical mirror planes[7], despite diffraction based measurements showing a crystallographic structure (point group *mmm*) that preserves them. This RA signal is already present at room temperature and is enhanced below the pseudogap temperature $T$*. To explain this data, it was proposed that there already exists a subtle monoclinic structural distortion at room temperature, and that a further inversion-breaking transition occurs at $T$*. The low temperature RA data could be fit to the coherent sum of a crystallographic *i*-type $C_2$-symmetric EQ term (point group 2/*m*) and a domain-averaged *c*-type $C_1$-symmetric ED term (point group 2′/*m* or *m*1′).

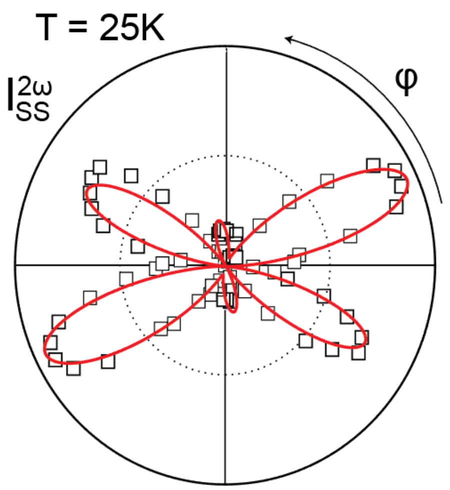


Figure S9: RA data from $YBa_2Cu_3O_{6.92}$ at $T$ = 25 K in the SS channel reproduced from Ref.[6]. The red curve is a fit the superposition of an *i*-type EQ term (*mmm*) and a *c*-type MD term (*mm*'*m*') from a single magnetic domain.

Here we show that the RA patterns from $YBa_2Cu_3O_y$ can also be explained by the presence of an inversion-preserving order parameter Φ of the type we report in $Sr_2CuO_2Cl_2$. In direct analogy to $Sr_2CuO_2Cl_2$, we fit the RA data from $YBa_2Cu_3O_y$ to the sum of a crystallographic *i*-type EQ term respecting the reported *mmm* point group, and a *c*-type MD term with a *mm′m′* point group from a single domain. In the SS channel, the functional form of the RA pattern is given by

$$I_{SS}^{2\omega} \propto |(a\cos^3\varphi\sin\varphi + b\ \cos\varphi\sin^3\varphi) + (c\cos^2\varphi + d\sin^2\varphi)|^2$$

where $a = \chi_{xyxy}^{EQ\,(i)} + \chi_{yxxy}^{EQ\,(i)} + \chi_{yyxx}^{EQ\,(i)} - \chi_{yyyy}^{EQ\,(i)}$, $b = \chi_{xxxx}^{EQ\,(i)} - 2\chi_{xxyy}^{EQ\,(i)} - \chi_{yxyx}^{EQ\,(i)}$, $c = \chi_{yyz}^{MD\,(c)}$ and $d = \chi_{xxz}^{MD\,(c)}$. As shown in Fig. S9, this also fits the $YBa_2Cu_3O_y$ data extremely well.

**Supplementary references**


1. Varma, C. M. Pseudogap and Fermi arcs in underdoped cuprates. *Physical Review B* **99**, 224516 (2019).
2. Birss, R. R. *Symmetry and magnetism*. (John Wiley & Sons, 1964).
3. Miller, L. L. *et al.* Synthesis, structure, and properties of $Sr_2CuO_2Cl_2$. *Phys. Rev. B* **41**, 1921–1925 (1990).
4. Sahota, D. G. *et al.* Many-body recombination in photoexcited insulating cuprates. *Phys. Rev. Research* **1**, 033214 (2019).
5. Hofmann, M. *et al.* Evidence for a large magnetic heat current in insulating layered cuprates. *Phys. Rev. B* **67**, 184502 (2003).
6. Jeong, J.-W., Shin, S.-C., Lyubchanskii, I. L. & Varyukhin, V. N. Strain-induced three-photon effects. *Phys. Rev. B* **62**, 13455–13463 (2000).
7. Zhao, L. *et al.* A global inversion-symmetry-broken phase inside the pseudogap region of $YBa_2Cu_3O_y$. *Nature Physics* **13**, 250–254 (2017).
